# Supplementary material for: Fine-Grained Modeling and Optimization for Intelligent Resource Management in Big Data Processing
Source: arXiv:2207.02026 source file (2022-07-09)
Supplement: Supplementary file 1 [file appendix_opt_bak.tex]

\section{Stage-level optimization}

In this section, we present our {\it Stage-level Optimizer (SO)} that minimizes both stage latency and cost based on instance-level models.

\begin{figure}[t]
	\centering
%	\vspace{-0.1in}
%	\hspace{-6cm}
  \includegraphics[height=4.5cm,width=.7\linewidth]{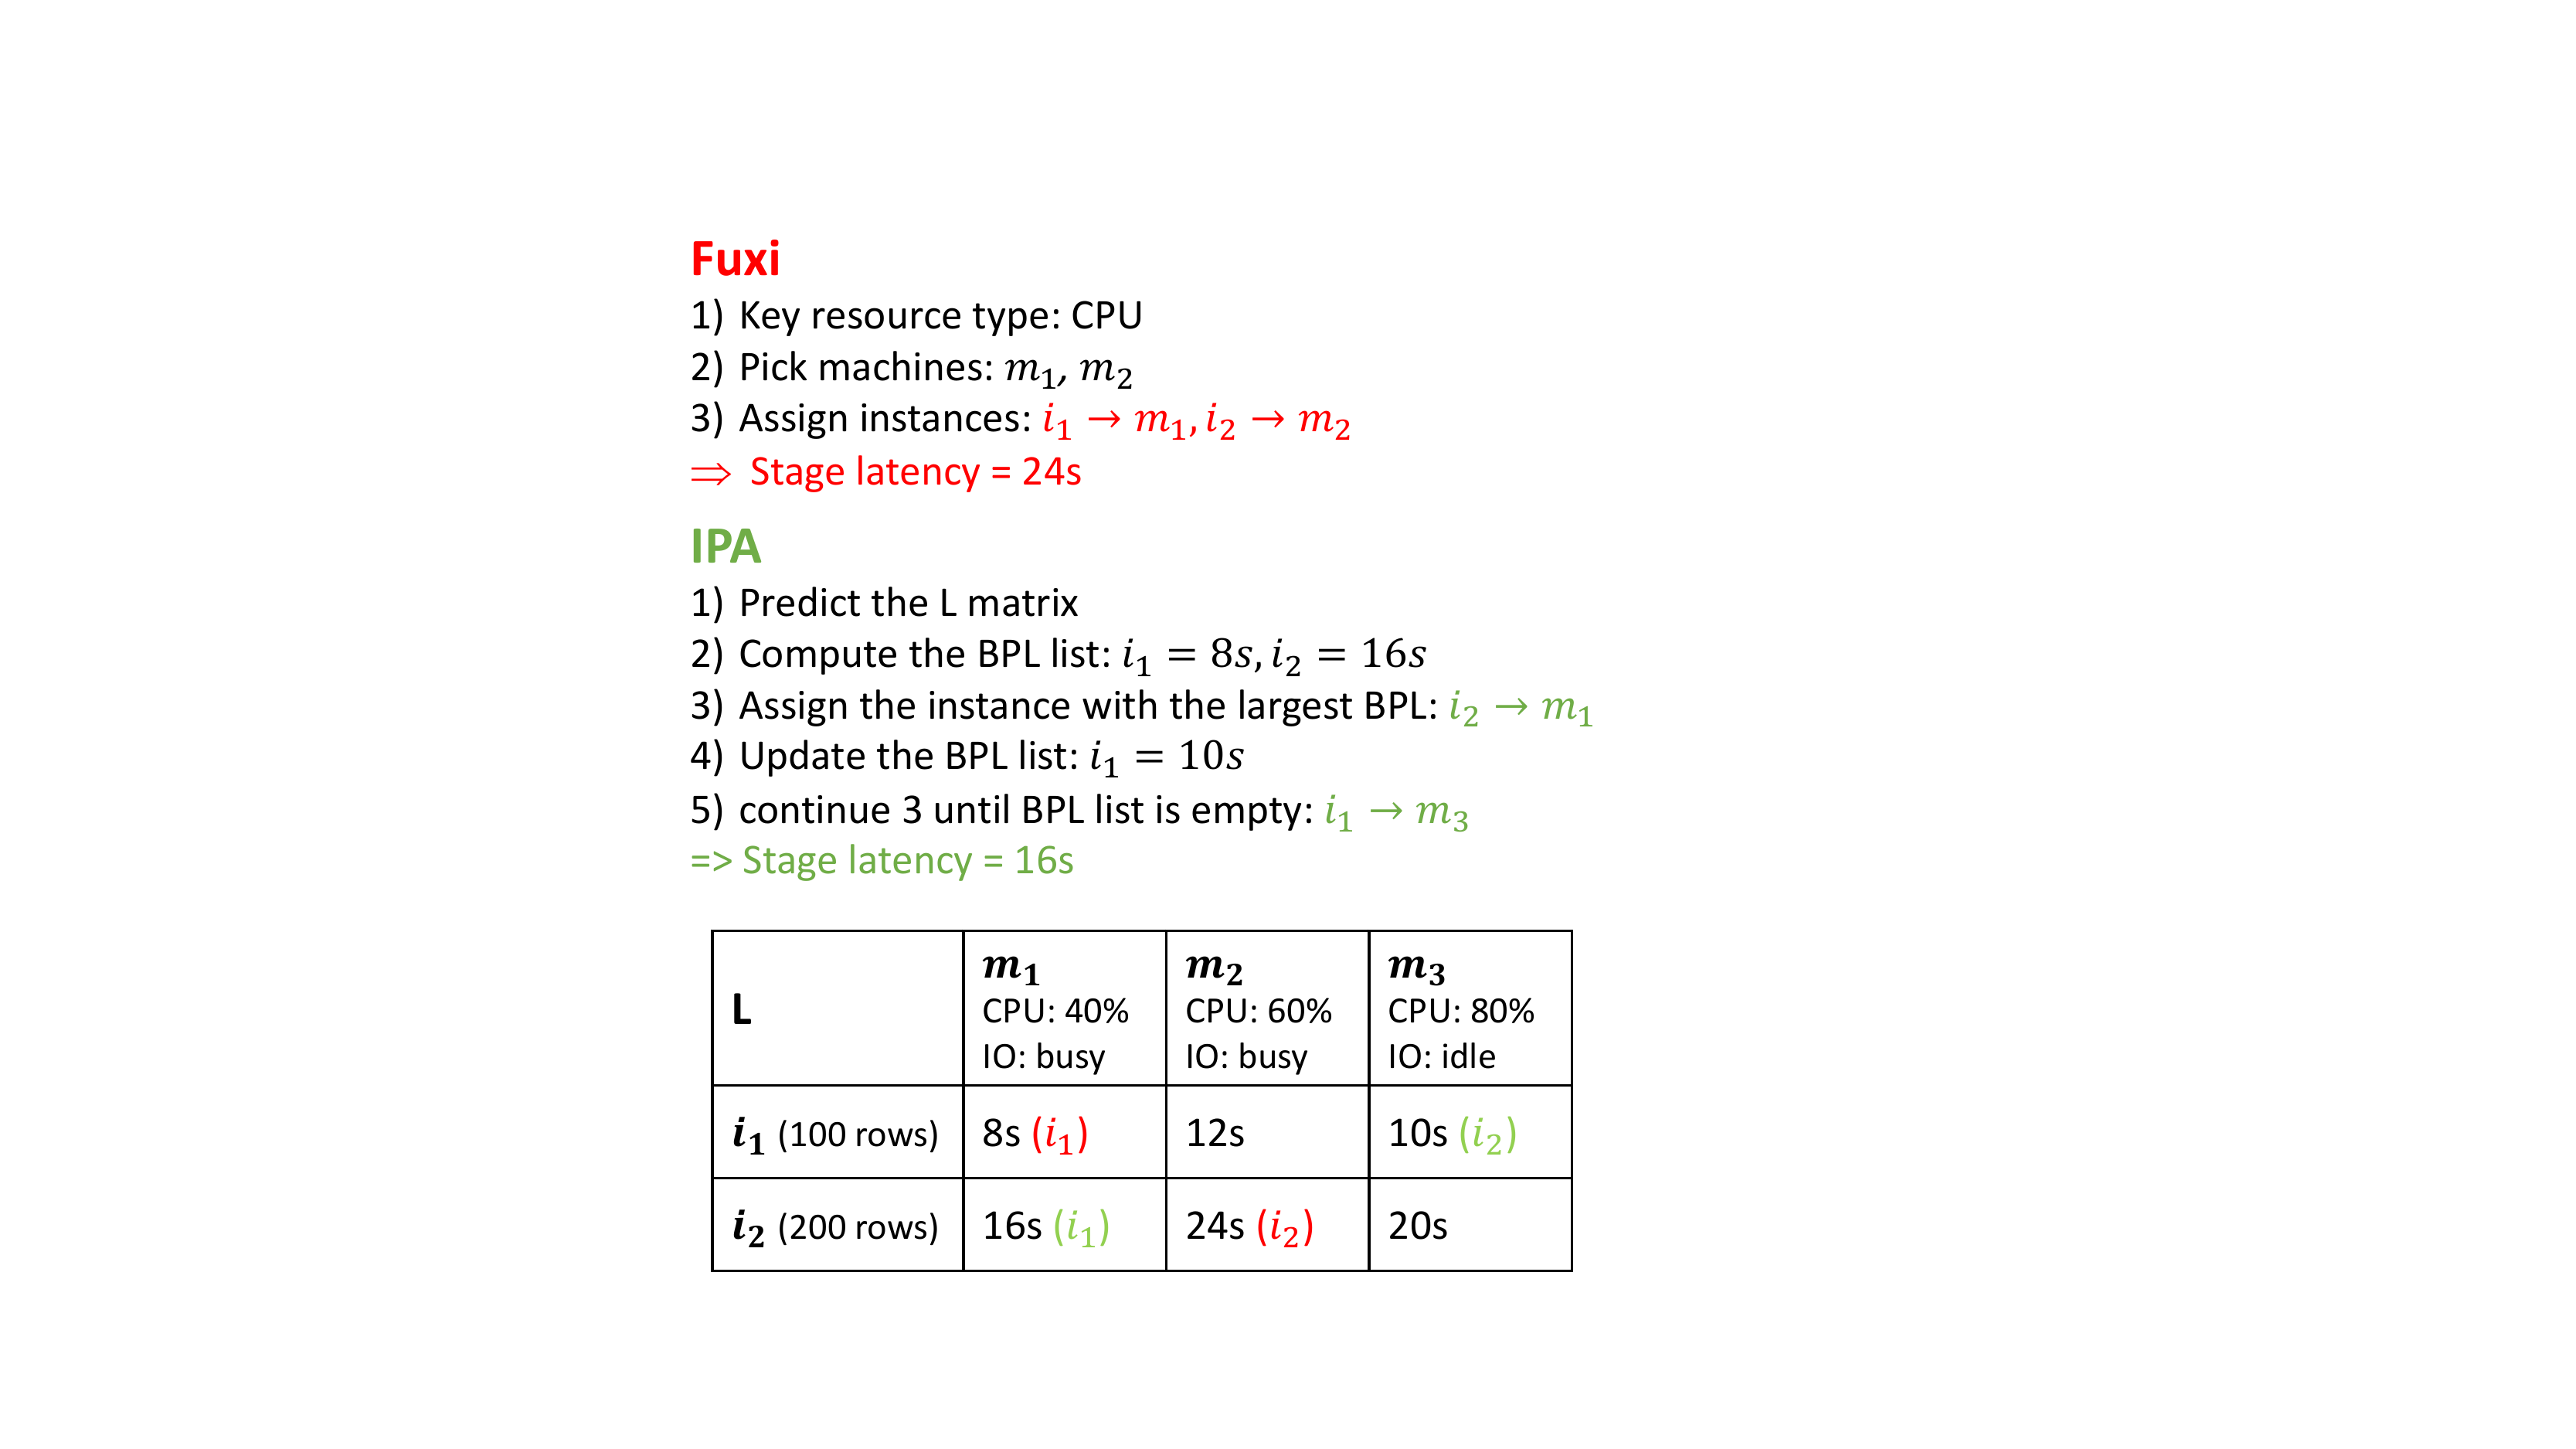}
  \vspace{-0.1in}
  \captionof{figure}{An example to compare Fuxi to an optimal solution \todo{typos for IPA solution. add RAA decisoin?}}
  \vspace{-0.1in}
  \label{fig:toy}
\end{figure}


%\begin{figure}[t]
%	\centering
%%	\vspace{-0.1in}
%%	\hspace{-6cm}
%\begin{minipage}{.5\linewidth}
%  \includegraphics[height=4.5cm,width=.95\linewidth]{figures/stage-profiling.pdf}
%  \captionof{figure}{Latency variation of 6716 instances in a stage}
%   \vspace{-0.1in}
%  \label{fig:inst-profiling}
%\end{minipage}%
%%\hspace{0.1in}
%\begin{minipage}{.5\linewidth}
%  \includegraphics[height=4.5cm,width=.95\linewidth]{figures/toy-example.pdf}
%  \captionof{figure}{A toy example}
%  \vspace{-0.1in}
%  \label{fig:toy}
%\end{minipage}%
%\end{figure}

%\subsection{Motivation}
%
%During job execution, the granularity of scheduling is a stage. Once a stage is handed to the scheduler, 
%it will make two decisions: the {\it placement plan (PP)}, which maps instances to machines, and the {\it resource plan (RP)}, which determines the CPU and memory resources in the container on the machine to which an instance is assigned.
%
%The Fuxi scheduler~\cite{fuxi-vldb14}, like most recent schedulers~\cite{Yarn,trident-vldb21} in big data systems, makes the placement plan decision by treating instances in a stage as blackboxes, oblivious of their workload characteristics or expected latencies. 
%For example, when resources are sufficient for a stage, Fuxi decides a placement plan for $m$ instances by the following steps: 
%(1) Identify the key resource in the current cluster, which is the bottleneck of the current cluster.
%(2) Pick $m$ machines\footnote{When the cluster has enough available machines, Fuxi has this diverse placement preference to send instances to different machines. 
%%Here we simplify the procedure by assuming available machines are sufficient.
%}, with top-$m$ lowest resource watermarks.
%(3) Assign instances, in order of their instance id, to the $m$ machines, and use the same resource plan for each instance as suggested by HBO.
%
%
%Although Fuxi's strategy could make a decision very efficiently at a milli-second level, it leads to suboptimal placement plans due to the negligence of latency variances among instances.
%%\todo{move the profiling example to the modeling section}
%\cut{
%To show an example of the latency variance, Figure~\ref{fig:inst-profiling} profiles a stage of 6716 instances sorted by (a) CPU utilization and (b) by input row number. %in a production workload. 
%Even though the instances share the same (sub)query structure and the same resource plan, the instances exhibit great variation of latencies, which could l be caused by different instance or machine characteristics.
%(1) For the instances running on machines with similar system states (e.g., same CPU utilization), their latency is positively correlated to the input row numbers. 
%(2) For those instances that run on machines with different CPU utilization, we observe that the latency has an increasing trend \todo{which is not visible in the current plot} as the CPU utilization rises up, which is due to lack of perfect isolation in big data systems.
%}

During job execution, once a stage is handed to the scheduler,  two decisions are made: 
the {\it placement plan (PP)}, which maps instances to machines, and the {\it resource plan (RP)}, which determines the CPU and memory resources in the container on the machine to which an instance is assigned.
The current Fuxi scheduler~\cite{fuxi-vldb14} decides a placement plan for $m$ instances as follows: 
(1) Identify the key resource in the current cluster, which is the bottleneck of the current cluster.
(2) Pick $m$ machines\footnote{When the cluster has enough available machines, Fuxi has this diverse placement preference to send instances to different machines. 
%Here we simplify the procedure by assuming available machines are sufficient.
}, with top-$m$ lowest resource watermarks.
(3) Assign instances, in order of their instance id, to the $m$ machines, and use the same resource plan for each instance as suggested by HBO.
However, its negligence of latency variance among instances leads to suboptimal decisions for PP and RP: 

\underline{Example 2.} %We next explain why neglecting instance latencies can lead to poor decisions for both placement plans and resource plans. 
Figure~\ref{fig:toy} shows how Fuxi gets a suboptimal placement plan in a toy example of sending a stage of 2 instances ($i_1$, $i_2$) to a cluster of 3 available machines ($m_1$, $m_2$, $m_3$).
Assume that the instance latency is proportional to its input row number on the same machine, and the current key resource in the cluster is CPU.
In this example, Fuxi first picks $m_1$ and $m_2$ as machines with the top-2 lowest CPU utilization (watermarks) and assigns $i_1$ and $i_2$ to them respectively. The stage latency, i.e., the maximum instance latency, is 24s.
However, the {\em optimal placement plan} could achieve a 16s stage latency by assigning $i_1$ to $m_3$ and $i_2$ to $m_1$ in this example.

Furthermore, the big variance in instance latencies also leads to
resource overusing based on the current resource plan. 
Like other resource optimizers in big data systems~\cite{cleo-sigmod20,qrop-icde18,udao-vldb19,spark-moo-icde21}, HBO recommends resource plans uniformly to each instance without considering the instance characteristics and machine states.
In our toy example, $i_1$ and $i_2$ share the same resource plan despite the differences in the data load. 
An {\em optimal resource plan} would be adding resources for $i_1$ and reducing resources for $i_2$ to reduce both latency and cost. However, assigning resources uniformly to all instances would miss the opportunity to minimize both objectives.

To address these issues, our stage optimizer (SO) employs a new {\it Intelligent Placement Advisor (IPA)}, which derives a  latency-aware placement plan to reduce the stage latency, and a novel {\it Resource Assignment Advisor (RAA)}, which derives instance-specific resource plans to further reduce latency and cost in a hierarchical MOO framework. Both methods are optimized to run under 100 msec.

%To address these issues, our stage optimizer (SO) could produce PP and RP to reduce both stage latency and cost within 100ms by using the {\it Intelligent Placement Advisor (IPA)} and the {\it Resource Assignment Advisor (RAA)}.
%IPA makes latency-aware placement plans to reduce the stage latency.
%And RAA makes instance-oriented resource plans to further reduce more latency and cost in a hierarchical MOO framework.
%An intuitive optimization would be adding resources for $i_1$ and reducing resources for $i_2$ to save more latency and cost. 
%However, assigning resource uniformly to all instances could miss the opportunity to minimize both objectives.
%Towards the challenges, SO produces PP and RP to reduce both stage latency and cost within 100ms by using the {\it Intelligent Placement Advisor (IPA)} and the {\it Resource Assignment Advisor (RAA)}.
%First, given the recommended RP from HBO (as the default RP), IPA will make a latency-aware placement plan to reduce the stage latency based on the fine-grained model. 
%And RAA makes instance-oriented resource plans to further reduce more latency and cost by solving a hierarchical MOO problem.

\subsection{Intelligent Placement Advisor (IPA)}

IPA takes the placement request with the MCI features of a stage from the scheduler, and returns a placement plan (PP) to reduce the stage latency. Note that PP does not change resource consumptions because all the instances are using the same resource plan at this phase. Therefore, we omit the discussion of reducing cost in IPA. Toward its goal, IPA feeds the MCI features to the latency model and builds a latency matrix to include the predictions of running the instances on all available machines. It then applies an approximate approach 
to solve the placement problem that is NP-hard in nature while meeting the stringent time constraint of  100msec.
%Indeed, it first extracts the MCI features and generates a latency matrix that involves the predictions of running instances on all available machines. Then it applies an approximate approach with instance and machine clustering to solve the placement plan as an NP-hard problem.

For the discussion below, we assume that the total available resources in a cluster are always more than a stage's need\footnote{Otherwise, there will be some scheduling delays before the stage arrives.}  once a stage is handed to IPA -- this assumption is likely to be met in a production environment with 10's thousands of machines.
Based on this assumption, we further suppose that %the scheduling delay is negligible compared to the stage latency, and 
all the instances of a stage can start running simultaneously and 
the stage latency is equal to the maximum instance latency.

\minip{Problem Setup.}
Consider the problem of sending 
a stage of $m$ instances $X=(x_1, ... , x_m)$, each with the identical demand of $d$ resource types ($r^1, r^2, ..., r^d$), to $n$  machines $Y=(y_1, ..., y_j, ..., y_n)$, each with the capacity of $d$ resources ($c_j^1, c_j^2, ..., c_j^d$). 
Further denote 
\begin{enumerate}
	\item $L\in \mathcal{R}^{m\times n}$ as the latency matrix, where $L_i^j$ is the latency of instance $x_i$ running over machine  $y_j$,
	\item $x_i \rightarrow y_j$ as sending the instance $x_i$ to the machine $y_j$,
	\item $P = \{x_i \rightarrow y_{p_i}, \forall i \in [1,m] | \, p_i \in [1, n]\}$ as the placement plan, and
	\item $B \in \mathcal{R}^{m\times n}$ as the binary matrix that codifies $P$, with $B_i^j = 1$ when $x_i \rightarrow y_j$. 
\end{enumerate}

Our goal is to minimize the stage latency, $\max_i L_i^{p_i}$, with a placement plan that meets the {\em resource capacity constraint} of each machine and a {\em diverse placement preference} (soft constraint) of sending instances to different machines to reduce resource contention. %(e.g., IO)

Denote $s_j$ as the maximum number of instances a machine $y_j$ can take based on the constraint and preference. We have 
\begin{equation}
s_j =  \min \{\lfloor c_j^1 / r^1 \rfloor, \lfloor c_j^2 / r^2 \rfloor, ..., \lfloor c_j^d / r^d\rfloor, \alpha \} 
\end{equation}
where $\alpha$ is a parameter that defines the maximum number of instances each machine can take based on the diverse placement preference. 
Basically, a smaller $\alpha$ shows a stronger preference of the diverse placement for a stage and we have $\alpha >= \lceil m/n \rceil$. 

Therefore, we formalize our problem as follows.
%\begin{align}
%    & \min_{P} (\max_i L_i^{p_i} ) \\
%    \mbox{s.t.} & \;\; count(P, j) \leq s_j, \forall j
%\end{align}
%where $count(P, j)$ returns the frequency of machine $y_j$ in the placement plan $P$.
%By codifying the placement plan using the binary matrix $B$, we rewrite the problem as 
\begin{align}
& \min_{B} (\max_{ij} L_i^j B_i^j ) \\
\mbox{s.t.} & \;\; \sum_i B_i^j = 1, \forall i  
\;\; \mbox{and}
\;\; \sum_j B_i^j \leq s_j, \forall j
%    \mbox{s.t.} & \;\; \sum_i B_i^j = 1, \forall i \\
%                & \;\; \sum_j B_i^j \leq s_j, \forall j
\end{align}

Since the variable $B$ is a binary matrix,  our problem is an NP-hard {\em Integer Linear Programming (ILP)}  problem \todo{citation}.


\minip{The approximate approach.}
%\label{sec:appr-algo}
%\noindent
%Recall that the available resources in a cluster are always more than a stage's need when the request is handed to IPA. We optimistically assume there must be sufficient feasible solutions to meet the constraints. E.g., the minimum stage latency is upper bounded by Fuxi's placement plan.
Since the stage latency is the maximum instance latency, intuitively, the placement plan wants to reduce the latency of the longer-running instances by sending them to the machines where they can run faster, potentially at the cost of 
compromising the latency of other short-running instances. %on other machines.

Based on this intuition, we design an approximate algorithm to solve the placement plan in IPA. 
We first prioritize the instances by their {\it best possible latency} (BPL), where BPL is defined as the minimum latency that an instance  can achieve among all available machines $Y^*$, e.g., $BPL_i = \min_{\{j | Y_j \in Y^* \}} L_i^j$. Then we keep sending the instance of the largest BPL to its matched machine and updating the BPL for instances when a machine cannot take more instances.

The full procedures of our approach are described as follows. \todo{Turn the steps below into a pseudocode.}

{\it Step 1.} Calculate the predicted latency matrix $L$ and the maximum number of instances accepted on each machine $s_j$.
% L O(mn) | embarrassingly parallel, GPU => O(mn/\verb|p|)
% S O(nd) | vectorizable => O(d)

{\it Step 2.} Initialize the available machines as $Y^* = Y$, instance remained to be sent as $X^* = X$, and the placement plan $P = \{\}$.
% O(1)

{\it Step 3.} Get the BPL for all the remaining instances to have a BPL list. $BPL_i = \min_{\{j | Y_j \in Y*\} } L_i^j, \forall i \in \{i | x_i \in X^*\}$
% O(mn) | vectorizable => O(n)

{\it Step 4.} Get the id $i_t = arg\max_{\{i | x_i \in X^*\}}(BPL_i)$ for the instance of the largest BPL.
% O(m)

{\it Step 5.} Get the id $j_t = arg\min_{\{j | Y_j \in Y*\} } L_i^j$ for the machine that achieves BPL with $x_{i_t}$.
% O(n)

{\it Step 6.} $P = P \bigcup \{x_{i_t} \rightarrow y_{j_t}\}$. Update $X^* = X^* - \{ x_{i_t} \}$, $s_j = s_j - 1$. 
% O(1)

{\it Step 7.} When $s_j$ equals 0, further update $Y^* = Y^* - \{ y_{j_t}\}$ and recalculate the BPL list. Otherwise, skip the step.
% 0 or O(m), at most n updates.

{\it Step 8.} When $X^*$ is empty, return P and finish. Otherwise, if $Y^*$ is empty, return ``no solution found'', else go back to step 4.
% m loops in total

\underline{Time Complexity}. The total time complexity is $O(m(m+n)+d)$ by using parallelism and vectorized computations in the implementation. 
\todo{Discuss the complexity of other packing algorithms to show that our complexity is lower, or do so after clustering.}
%\todo{merge the algorithm and complexity analysis into a table with two columns if time permits}

\minip{Boost IPA with clustering.} %\noindent
A remaining issue is that in the production workload, a stage can be up to 80K instances, and the number of available machines  can also be tens of thousands. 
For example, solving the placement plan for a stage of 6716 instances (Figure~\ref{fig:inst-profiling}) over 8000 available machines cost 2.366s. 
%2.366s = 1.840s (modeling) + 0.526s (solving)
However, a scheduler shall give the response within 100msec. %well under a second (cost 0.018s by Fuxi).
To further reduce the time cost, we exploit the idea that among large numbers of machines and instances, groups of machines or groups of instances may behave similarly in the placement problem. Therefore, we 
boost the IPA efficiency by clustering both machines and instances without losing much stage latency performance. 
%Towards the same stage, the solving time reduces to 0.054s (including 0.028s for modeling) with clustering.
%0.054s = 0.037s (modeling) + 0.017s (solving)

While there are many existing clustering methods \todo{cite}, running them on many instances with large MCI feature vectors is still an expensive operation. This motivates us to design a customized clustering method based on their MCI properties. An instance in a stage is characterized by its query plan (Ch1), instance meta (Ch2), its resource plan (Ch3) and additional instance meta (AIM).
When solving the placement plan, instances share the same Ch1 and Ch3 and can be characterized by Ch2 and AIM. 
Notice the time complexity of a clustering method is quadratic against the dimension of the instance data (considering the distance function as the Euclidean distance). Hence we want to shrink Ch2 and AIM to reduce the cost. 
Recall AIM fully depends on Ch1 and Ch2, and the two features in Ch2, the input row number and the input size, are proportional or positively related towards the same stage. 
Therefore, we approximately characterize an instance only by its input row number, and apply a 1D clustering algorithm on it.
In our work, we use a density-based clustering\todo{cite a textbook} that calculates the kernel density estimation (KDE) of the inputs in the 1D space, and uses the minimas of the density distribution as the boundaries to divide instances into clusters.
To represent a cluster, we choose the instance with largest input row number in the cluster to avoid latency underestimations.

A machine in the cluster is characterized by its system states (Ch4) and the hardware type (Ch5). While normally Ch5 only has fewer unique choices in a cluster, % at most 6 choices observed in our workloads.
the count-based features in Ch4, such as CPU utilization, could be infinite. 
Our model profiling results show that discretizing the system states properly only slightly impacts the model performance \todo{forward to the expr}.
Therefore, we discrete the Ch4 into a finite set and group machines with the same Ch4 and Ch5 values into the same cluster.
Consequently, machines in the same group have the same Ch4 and Ch5.

Assume after the clustering, we got $m'$ instance clusters $X^c=[X_1^c, X_2^c, ..., X_{m'}^c]$ and $n'$ machine $Y^c=[Y_1^c, Y_2^c, ..., Y_{n'}^c]$. Denote $\hat{X_i}^c$ and $\hat{Y_j}^c$ as the representatives for $X_i^c$ and $Y_i^c$, and we get $\hat{X}^c = [\hat{X_1}^c, \hat{X_2}^c, ..., \hat{X_3}^c]$, $\hat{Y}^c = [\hat{Y_1}^c, \hat{Y_2}^c, ..., \hat{Y_3}^c]$ as representative instance and machine lists.

Our approximate approach can be boosted by clustering with several changes. 
\todo{Wite the pseudocode but leave it to the appendix. The text needs only to highlight the differences, e.g., step 6. }

{\it Step 0.} Clustering instances and machines to get $X^c$ and $Y^c$ and $\hat{X}^c$ and $\hat{Y}^c$.
% O(mlogm + nlogn) -- distribute items to groups need a sort-based method

{\it Step 1.} Calculate the latency matrix $L$ against $\hat{X}^c$ and $\hat{Y}^c$. Calculate $s_j = \sum_{\{ j' | y_{j'} \in Y_{j}^c \}}{s_j'}, \forall j \in [1, n']$ as the maximum instances $Y_j^c$ can take, and $\beta_{i} = |X_i^c|$ as the number of instances in $X_i^c$.

{\it Step 2.} Initialize the available machines as $Y^* = \hat{Y}^c$, instance remained to be sent as $X^* = \hat{X}^c$, and the placement plan $P = \{\}$.

{\it Step 3-5.} keep the same steps to find the $i_t$ and $j_t$ over clusters.

{\it Step 6.} Get the number of instance can be sent $\delta = \min (\beta_{i_t}, s_{j_t})$ as minimum value between the number of instances in the instance cluster $X^c_{i_t}$ and the number of available machines in the machine cluster $Y^c_{j_t}$. Pick $\delta$ instances with top-$\delta$ input row numbers from $X^c_{i_t}$ as $X^\delta$ and $\delta$ machines from $Y^c_{j_t}$ as $Y^\delta$. 
Update $P = P \bigcup \{X^\delta_k \rightarrow Y^\delta_k |k\in [1,\delta] \}$.
Update $s_{j_t} = s_{j_t} - \delta$, $\beta_{i_t} = \beta_{i_t} - \delta$, $X^c_{i_t} = X^c_{i_t} - X^\delta$, $Y^c_{j_t} = Y^c_{j_t} - Y^\delta$.
% O(1) vectorizable for the place \delta pairs.

{\it Step 7-8.} keep the same steps.

The time complexity is $O(mlogm + nlogn + m'(m'+n') + d)$. Consider $m' \ll m, n' \ll n$ when $m$ and $n$ are thousands. The time complexity for a stage of large number of instances reduces to $O(mlogm + nlogn)$.
\todo{Explain where  $O(mlogm + nlogn)$ come from}

It is worth mentioning that instances in the same cluster can still have smaller variances due to the differences in input row numbers. 
To avoid the case when the number of machines is not enough for running the entire instance cluster while the longer-running instances cannot be sent in step 6, 
our approach gives instances with a larger input row number a higher priority to be chosen in the same group. It also sorts the instances in the descending input row number order during clustering to reduce the time complexity during picking instances from the cluster.
\todo{move to appendix.}

\cut{
	\begin{algorithm}[t]
		\caption{Approximate Approach}
		\label{alg:appr}
		\small
		\begin{algorithmic}[1]  
			\REQUIRE {latency matrix $L$ with size $(m, n)$, \\ resource plan matrix $R$ with size $(m, 2)$, \\ capacity matrix $C$ with size $(n, 2)$, \\ the maximum number of instances a machine can take $s$.}
			
			{\ }\\
			\underline{{Initialization Step:}}
			\STATE $B \leftarrow 0_{m\times n}$, $w \leftarrow 0_n$
			\STATE $L_{min} \leftarrow [\min L_{1, *}, \min L_{2, *}, ..., \min L_{m, *}]$
			\STATE $P \leftarrow argsort (L_{min}, ascent=False)$ 
			
			{\ }\\
			\underline{{Machine Picking Step:}}
			\REPEAT
			\STATE $i \leftarrow P.pop()$
			\STATE $J_{avail} = FilterAvailableMachines(R_{i,*}, C_{i,*}, w, s)$
			\STATE $L'_{i, *} = [L_{i, j} | j \in J_{avail}]$
			\IF {$L'_{i,*}.isEmpty()$}
			\STATE \Return{"NSF"}
			\ENDIF
			\STATE $j \leftarrow argmin(L'_{i,*})$
			\STATE $B_{i,j} \leftarrow 1$
			\FOR{$k \leftarrow 1$ to $2$}       
			\STATE $C_{j, k} \leftarrow C_{j, k} - R_{i, k}$
			\ENDFOR
			\STATE $w_j \leftarrow w_j + 1$
			\UNTIL{$P.isEmpty()$}
			\STATE \Return{$B$}
		\end{algorithmic}
	\end{algorithm}
}

\subsection{Resource Assignment Advisor (RAA)}

RAA tunes the resource plan of each instance to solve a MOO problem, e.g., minimizing both the stage latency and cost (CPU-hour) by increasing the resources for long-running instances and decreasing the resources for short-running instances after the placement plan after getting the placement plan from IPA.


\minip{Fast hierarchical MOO solution.}
RAA recommends the resource plans for each instance in the following 4 steps.

{\it Step 1: Instance clustering.} 
After instances are paired with machines, machine characteristics shall also be considered for instance clustering. 
RAA applies an inherent-based clustering strategy that can summarize new instance clusters from IPA's instance clusters without additional time overhead.
Specifically, we break up each instance cluster in IPA into separate new clusters when they are sent to different machine clusters. 
Notice that the breakup naturally happens at step 6 when $\delta$ instances are sent to machines belonging to the same cluster. 
Therefore it charges no additional time to generate new clusters and find the instance with the largest input row number as its representative.


{\it Step 2: Instance-level MOO.} 
Our previous work UDAO~\cite{spark-moo-icde21} proposed a Progressive Frontier (PF) approach that could minimize multi-objectives under stringent time requirements. PF requires differentiable models that can map configurations to objectives.
Towards our problem, RAA ensembles two objective models (one for instance latency, one for cost) based on the fine-grained instance latency model, and treats the resource plan (CPU cores and memory sizes) as the configuration to fit PF algorithm.
By applying PF (in parallel), RAA gets the Pareto-optimal solutions\footnote{the latency of the instance cluster equals the latency of the representative instance; the cost of a cluster is the cost of the representative times the cluster size} for each instance cluster efficiently. 


{\it Step 3: Stage-level MOO.} 
With a set of instance-level Pareto sets, RAA further constructs a stage-level Pareto set to minimize the stage-level latency (the maximum of instance latencies) and the stage-level cost (the summation of instance costs).
We define the {\it RAA path} shortly. %in Section~\ref{sec:raa-path}.
Along the trail of the RAA path, RAA efficiently finds the resource plan for each instance cluster from its instance-level Pareto set, and finds all Pareto-optimal solutions towards the stage. 
Instances from the same cluster are assigned with the same resource plan.
\todo{Is this as general as Qi's original algorithm?}

{\it Step 4: Resource plan recommendation.}
After getting the stage-level Pareto set from step 3, we reuse UDAO's Weighted Utopia Nearest (WUN) strategy to recommend the resource plans. 
WUN computes a weight vector for latency and cost based on previous traces to address their importances.
It recommends the resource plans whose objectives could achieve the smallest distance to Utopia with the importance weights.


\minip{RAA path.}\label{sec:raa-path.}
We now define the problem of how to construct a stage-level Pareto set from a set of instance Pareto sets. 

Without further notation, we use the term ``instance'' for ``instance cluster'' in the RAA path discussion.
Given $m$ instance-level Pareto sets, where each instance $i$ has $p_i \geq 1$ Pareto solutions, consider:

\begin{itemize}
	\item $\theta_i = [\theta_i^1, \theta_i^2,..., \theta_i^{p_i}], \forall i \in [1, m]$ as a list of resource plans that achieves Pareto-optimal solutions for instance $i$, where $\theta_i^{j}$ is a resource plan of CPU and memory sizes.
	\item $f_i = [f_i^{\theta_i^1}, f_i^{\theta_i^2}, ..., f_i^{{\theta_i^{p_i}}}], \forall i \in [1, m]$ as a list of Pareto-optimal solutions for instance $i$, where $f_i^{\theta_i^j} = (l_i^{\theta_i^j}, o_i^{\theta_i^j})$ is the Pareto solution of latency and cost. Denote $l_i = [l_i^{\theta_i^1}, l_i^{\theta_i^2}, ..., l_i^{{\theta_i^{p_i}}}]$.
	\item $\Theta_k = [\theta_1^{k_1}, \theta_2^{k_2}, ..., \theta_m^{k_m}]$ as the resource plans that achieves the $k^{th}$ stage Pareto-optimal solution, where $\theta_i^{k_i} \in \theta_i$.
	\item $F^{\Theta_k} = \Phi(\Theta_k) = (\max_i l_i^{\theta_i^{k_i}}, \sum_i o_i^{\theta_i^{k_i}})$,  $\forall i \in [1, m]$ is the $k^{th}$ stage Pareto-optimal solution, where $\Phi$ is the function mapping from resource plans to the two stage-level objectives
	\item $\Theta = [\Theta_1, \Theta_2, ...]$ is the a set of resource plans that achieve stage Pareto-optimal solutions.
	\item $F = [F^{\Theta_1}, F^{\Theta_2}, ...]$ is the stage-level Pareto-optimal solutions.
	\item $\lambda = [\lambda_1, \lambda_2, ..., \lambda_m]$ as a state, such that $\Theta^\lambda = [\theta_1^{\lambda_1},  \theta_2^{\lambda_2}, ..., \theta_m^{\lambda_m}]$.
	\item $\pi_i: \lambda \rightarrow \lambda'$ is a {\it step} such that $\lambda'_{i} = \lambda_i+1$ and $\lambda'_{i'} = \lambda_{i'}$ when $i' \neq i$
\end{itemize}


\begin{figure}[t]
	\centering
	\includegraphics[width=.48\textwidth]{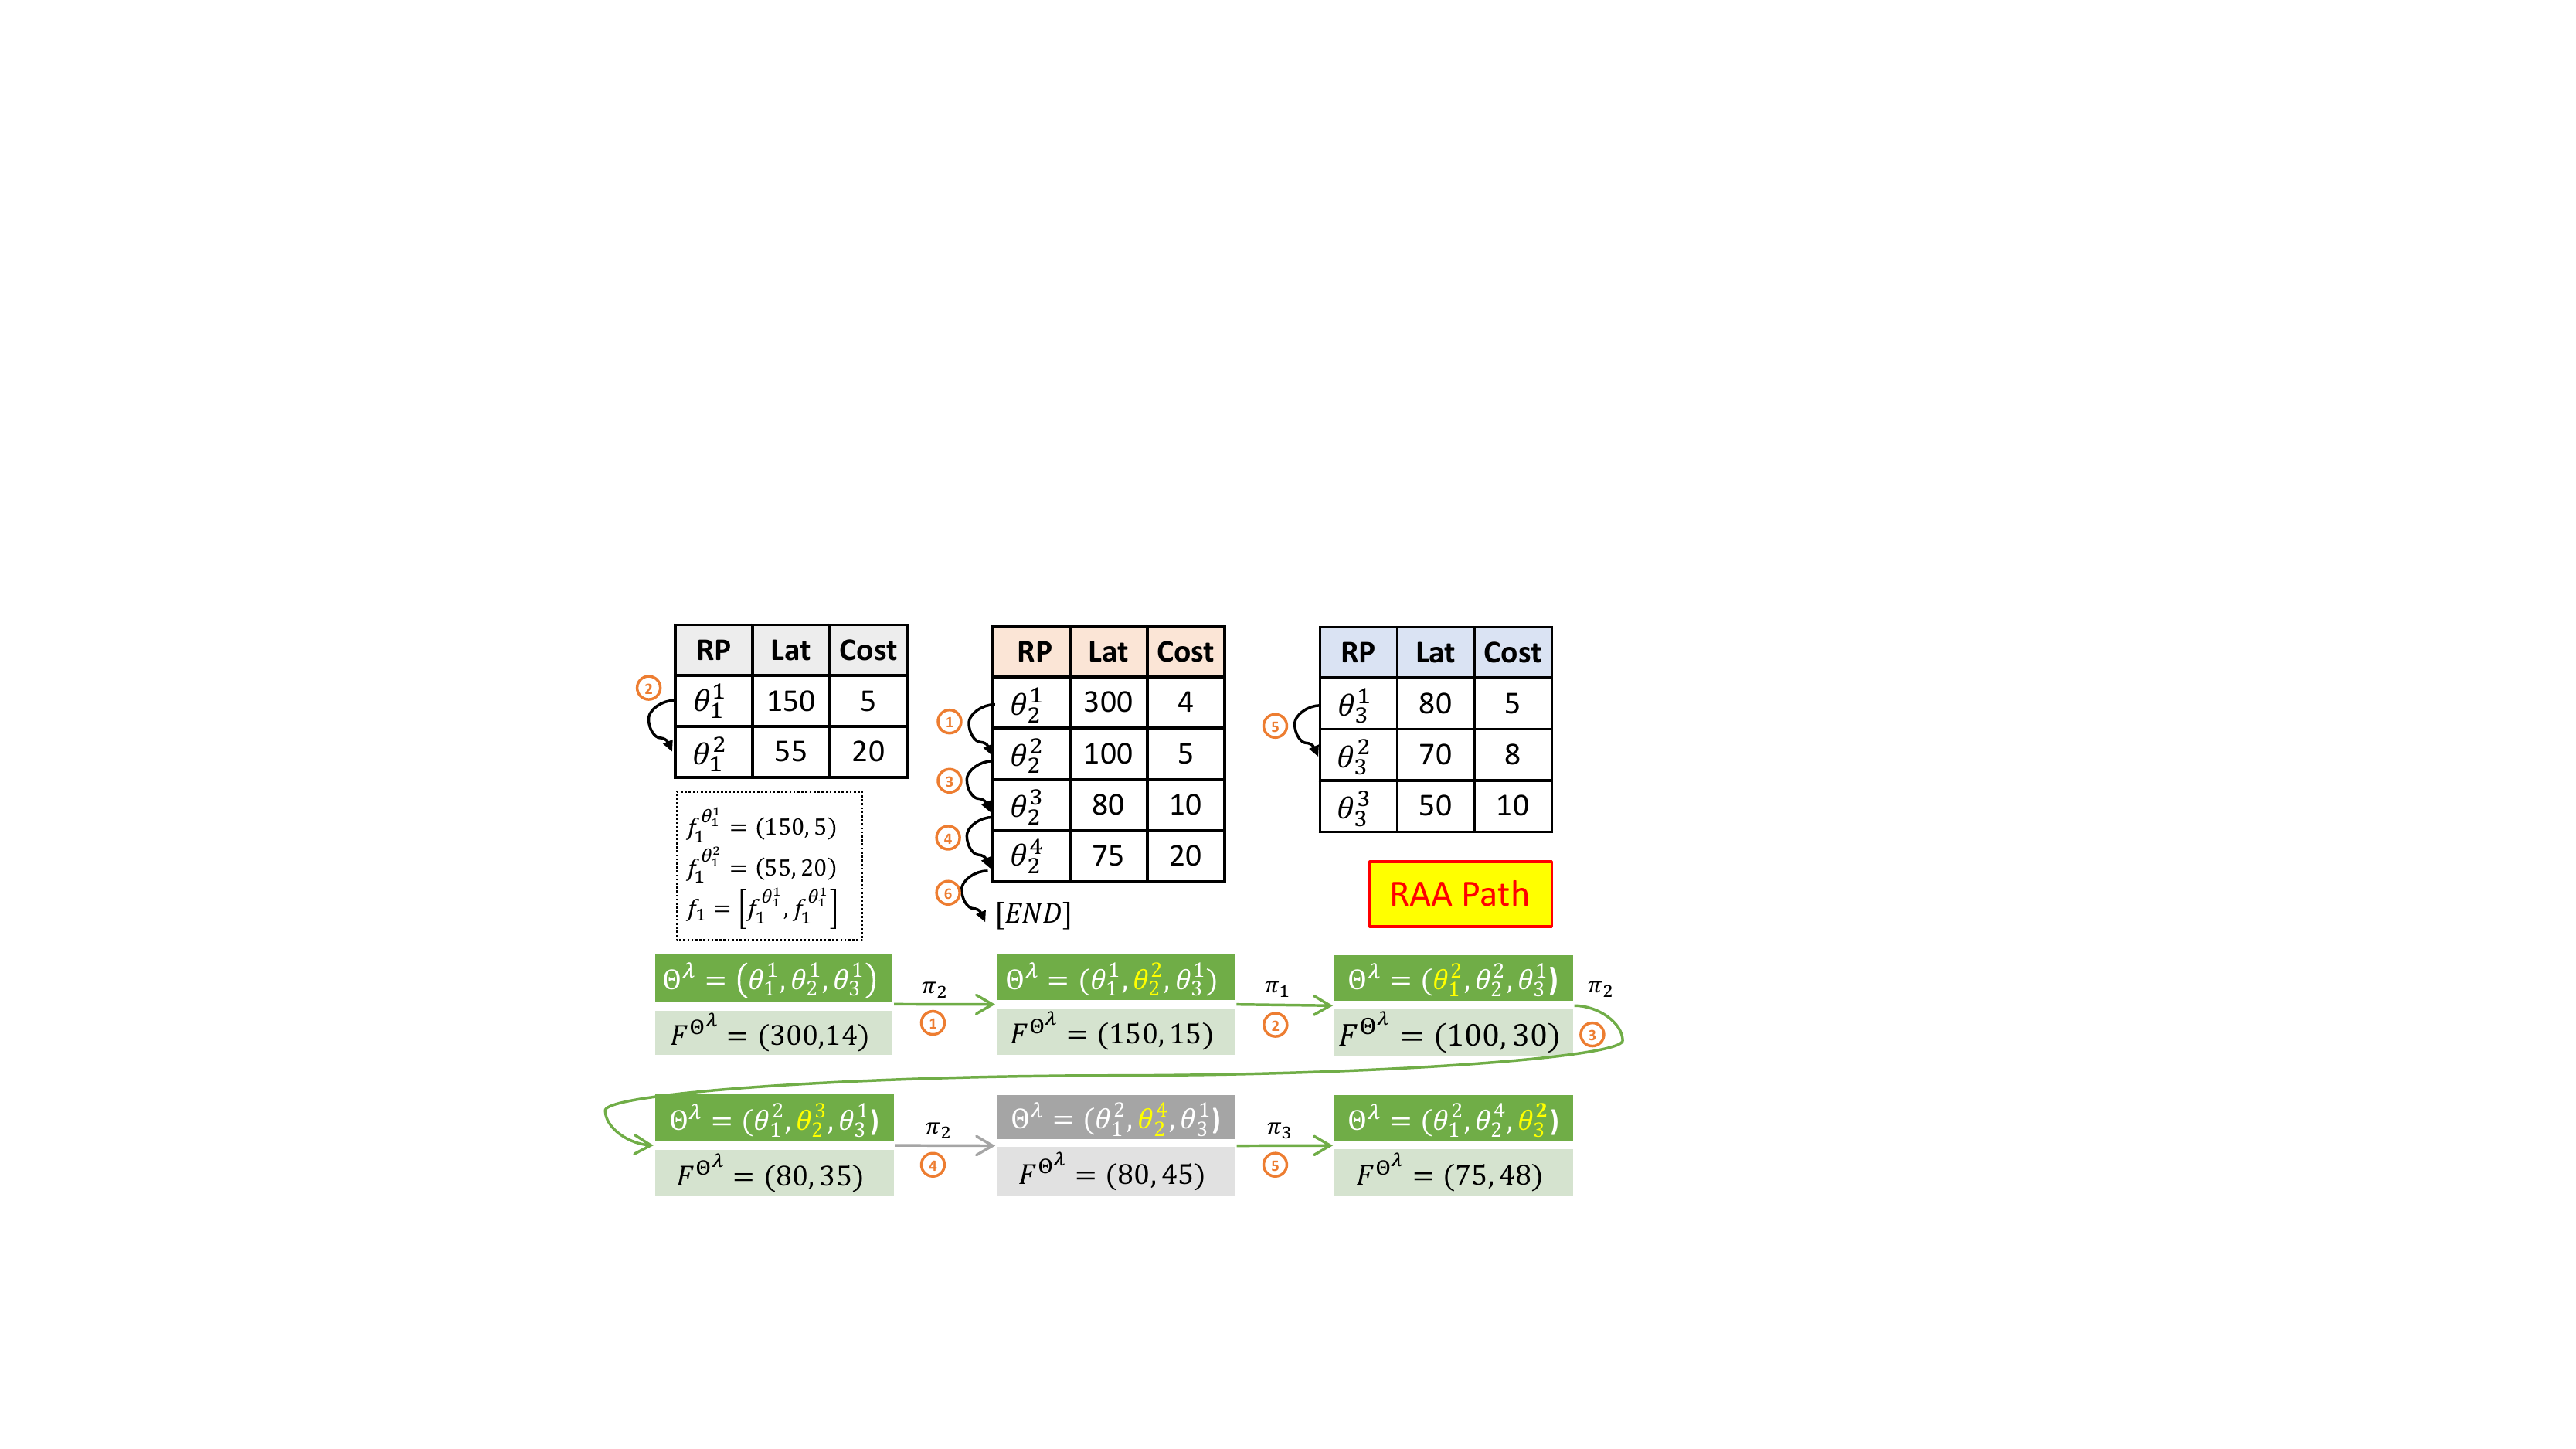}
	\vspace{-0.3in}
	\caption{RAA path example} %Machine system states trends in a representative cluster
	\vspace{-0.2in}
	\label{fig:raa-path}
\end{figure}

Notice PF algorithm generates Pareto-optimal solutions progressively, we get the Pareto $f_i$ sorted by one objective. WLOG, we assume each $f_i$ is listed with the descending order of latency, and hence the ascending order of cost.

Figure~\ref{fig:raa-path} shows an example of 3 instance Pareto set in a stage, where each instance has 2, 4, 3 Pareto-optimal solutions and each solution is sorted by latency in the descending order.

\begin{algorithm}[t]
	\caption{RAA path policy to construct $\Theta$ and $F$}
	\label{alg:appr-raa}
	\small
	\begin{algorithmic}[1]  
		\REQUIRE {$p_i, \theta_i, l_i$, $\forall i\in [1,m]$}.
		\STATE $\Theta = [], F=[], \lambda = [1, 1, ..., 1]$, smax=inf %Initialize Pareto Set:
		\STATE Build the max heap $Q$ with data points $[(l_i^1, i)], \forall i \in [1,m]$. % O(mlogm)
		\REPEAT
		\STATE qmax, $i = Q.pop()$ % O(1)
		\IF {qmax < smax}
		\STATE $\Theta.append(\Theta^\lambda)$
		\STATE $F.append(\Phi(\Theta^\lambda))$
		\STATE smax = qmax
		\ENDIF
		\STATE $\lambda = \pi_i(\lambda)$
		\IF {$\lambda_i > p_i$}
		\STATE \Return{$\Theta$, $F$}
		\ENDIF
		\STATE $Q.push((l_i^{\lambda_i}, i))$ %O(logm)
		\UNTIL{True}
	\end{algorithmic}
\end{algorithm}

Intuitively, if we are sure that one Pareto-optimal solution for the stage is bounded by a specify instance $i$ with a specific resource plan $\theta_i^j$ with the stage latency as $l_i^{\theta_i^j}$. 
To achieve the stage-level Pareto-optimality, for each of any other instance $i'$, we shall pick a resource plan $\theta_{i'}^{j'} \in \theta_{i'}$ with the maximum achievable latency without exceeding $l_i^{\theta_i^j}$, to minimize the cost usage.

Algorithm~\ref{alg:appr-raa} defines the RAA path policy that can effectively collect all the stage-level Pareto points with a set of steps. 
RAA shows its steps by iterating all the possible stage-level latency in the the descending order by choosing the resource plan for each instance from their Pareto sets.
To effectively achieve the iteration, we start by collecting all the largest latencies over all instances and constructing a max-heap over (latency, instance id) pairs with the latency order (line2).
After the max-heap pops a pair for the instance whose latency is the stage latency, we will push the next largest latency of the instance from its Pareto set back to the max-heap. 
We also maintains the smallest latency in the stage Pareto set during the path, and will append the stage Pareto when the stage latency decreases.

Figure~\ref{fig:raa-path} shows an example of RAA path, which could effectively iterate the possible stage-level latencies in a decreasing order by choosing the resource plan for each instance from their Pareto sets.

The time complexity of the algorithm is $O((m + \sum_i{p_i})logm)$. 
%The proof of the correctness is shown in our extension version \todo{cite extension}



%\todo{define the Pareto Point collection}

% \todo{a proof in the verbose version after submission}
% Assume the first non-Pareto point is from the state i s_i, check s_{i-1} and induce to a contradiction.
