# Supplementary material for: Fine-Grained Modeling and Optimization for Intelligent Resource Management in Big Data Processing
Source: arXiv:2207.02026 source file (2022-07-09)
Supplement: Supplementary file 2 [file appendix_raa_tmp.tex]

\section{Appendix on RAA}
\label{appendix-raa}
\underline{Example.} In Figure~\ref{fig:raa-example}, we have $f_1$ as the predictive model for latency and  $f_2$ for cost. Also we have $g_1 = max$ and $g_2 = sum$. Suppose we pick up $[\theta_1^1 ,\theta_2^2]$ as the stage-level resource configuration.  

In the upper left Table of Inst 1, from the row indexed by $\theta_1^1$ we know that $f_1(\theta_1^1)=150$, and $f_2(\theta_1^1)=5$. Similarly from Table of Inst 2 we have $f_1(\theta_2^2)=100$, and $f_2(\theta_2^2)=5$. 

Now we can compute the stage-level objectives using $g_1=max$ and $g_2=sum$.  More specifically, we have $F_1 = g_1(f_1(\theta_1^1), f_1(\theta_2^2)) = max(150, 100) = 150$, and $F_2 = g_2(f_2(\theta_1^1), f_2(\theta_2^2)) = sum(5, 5) = 10$. 

Hence the stage-level solution corresponding to $[\theta_1^1 ,\theta_2^2]$ is $[150 ,10]$.


\proposition \label{algo2_optimality} For a stage-level MOO problem as we defined, Algorithm~\ref{algo_stage_moo} guarantees to find a subset of stage-level Pareto optimal points. 
